# Supplementary material for: Good-for-MDPs Automata for Probabilistic Analysis and Reinforcement Learning
Source: arXiv:1909.05081 source file (2019-10-30)
Supplement: Supplementary file 1 [file appendix.tex]

%%% Local Variables:
%%% mode: latex
%%% TeX-master: "main.tex"
%%% TeX-PDF-mode: t
%%% End:
